# Supplementary material for: FLSys: Toward an Open Ecosystem for Federated Learning Mobile Apps
Source: arXiv:2111.09445 source file (2023-03-11)
Supplement: Supplementary file 1 [file sec9_appendix.tex]

\section{Differential Privacy Mechanisms}
\label{appendix_DP}

Differential privacy (DP)~\cite{dwork-DP-def4,dwork-DP-definition,dwork-DP-def2,dwork-DP-def3} offers a state-of-the-art metric for quantifying privacy when sensitive data are involved, and it is currently deployed by organizations such as Apple, Google, Microsoft, Facebook, and US Census Bureau~\cite{DP-cryptography}. An algorithm satisfies DP when adding, removing, or changing one record does not alter its output. The definition of DP was formalized by~\cite{dwork-DP-definition} as follows: 

\begin{definition}[Differential Privacy \cite{dwork-DP-definition}]
\label{def_DP}
A randomized mechanism $\mathcal{M}: \mathcal{D} \to \mathcal{R}$ with domain $\mathcal{D}$ and range $\mathcal{R}$ fulfills $(\varepsilon, \delta)$-differential privacy if for any two neighboring datasets $(d, d') \in \mathcal{D}$ that differ exactly in a single data sample and for any subset of outputs $S \in \mathcal{R}$, the following condition holds:
\begin{equation}
\tag{A.1}
Pr[\mathcal{M}(d) = S] \leq e^\varepsilon Pr[\mathcal{M}(d') = S] + \delta
\end{equation}
\end{definition}

\noindent
where $Pr$ stands for probability, $\varepsilon$ is the privacy budget and $\delta$ is the probability that $\varepsilon$-differential privacy is broken. 
The privacy budget $\varepsilon$ controls the amount of difference between the probability distributions generated by $d$ and $d'$. The smaller value of $\varepsilon$, the stronger privacy guarantee. 

In this article, we tested FLSys with two well-known DP mechanisms for FL: user-level DP (User-DP)~\cite{mcmahan-userDP} and sample level local DP (LDP)~\cite{LDP1,LDP2,LDP3,kim2021federated}. 

User-DP guarantees to protect clients' participation (membership) information in training the global model. User-DP is implemented by clipping local gradients~\cite{pascanu2013gradclipping} derived from clients' local training data. Then, DP-preserving noise in added into the aggregation of the clipped local gradients (using federated averaging algorithm~\cite{mcmahan-fedavg}).

\begin{definition}[User-level Differential Privacy \cite{mcmahan-userDP}]
\label{def_userDP}
A randomized mechanism $\mathcal{M}: \mathcal{D} \to \mathcal{R}$ with domain $\mathcal{D}$ and range $\mathcal{R}$ fulfills $(\varepsilon, \delta)$-differential privacy at user level if for any two neighboring sets of users $(u, u')$ that differ in exactly one user, $(\mathcal{D}_u, \mathcal{D}_{u'}) \in \mathcal{D}$ and for any subset of outputs $S \in \mathcal{R}$, the following condition holds:
\begin{equation}
\tag{A.2}
Pr[\mathcal{M}(\mathcal{D}_u) = S] \leq e^\varepsilon Pr[\mathcal{M}(\mathcal{D}_{u'}) = S] + \delta
\end{equation}
\end{definition}

In LDP, one focuses on protecting the legitimate value of a training sample of an individual user. The definition of LDP is as follows:

\begin{definition}[Local Differential Privacy]
\label{def_LDP}
A randomized mechanism $\mathcal{M}$ satisfies $(\varepsilon, \delta)$-LDP if for any two inputs $(x, x')$ and for any subset of outputs $S \in Range(\mathcal{M})$, the following condition holds:
\begin{equation}
\tag{A.3}
Pr[\mathcal{M}(x) = S] \leq e^\varepsilon Pr[\mathcal{M}(x') = S] + \delta
\end{equation}
\end{definition}
  \vspace{-0.25in}
